# Supplementary material for: Understanding the Impact of Adversarial Robustness on Accuracy Disparity
Source: arXiv:2211.15762 source file (2023-05-28)
Supplement: Supplementary file 1 [file supp.tex]

\documentclass{article}
\usepackage{amssymb}
\usepackage[utf8]{inputenc} %
\usepackage[T1]{fontenc}    %
\usepackage{hyperref}       %
\usepackage{url}            %
\usepackage{booktabs}       %
\usepackage{amsfonts}       %
\usepackage{nicefrac}       %
\usepackage{microtype}      %

\usepackage{amsmath,amsbsy,amsfonts,amssymb,amsthm,dsfont,units}
\usepackage{cleveref}
\usepackage{tabularx}
\usepackage{graphicx}
\usepackage{makecell}
\usepackage{delarray}
\usepackage{times}
\usepackage{mathrsfs}
\usepackage{authblk}
\usepackage{algorithm,mathtools}
\usepackage{algorithm, algorithmicx}
\usepackage[noend]{algpseudocode}
\usepackage[nonatbib]{neurips_2022}
\usepackage{color,cases}
\usepackage{tikz}
\usepackage{xspace}
\usepackage{enumerate}
\usepackage{algorithm}
\usepackage{nameref}
\usepackage{booktabs}
\usepackage{mdframed}
\usepackage{fmtcount}
\usepackage[super]{nth}
\usepackage{footnote}
\usepackage{bbm}
\usepackage{thmtools,thm-restate}
\usetikzlibrary{calc,shapes}
\usepackage{subcaption}
\usepackage{hyperref}
\usepackage{empheq}

\usepackage{multirow}
\usepackage{enumitem}

\usepackage[maxbibnames=99, backend=bibtex]{biblatex}
\addbibresource{references.bib}

 \newcommand{\IGNORE}[1]{}

\newcommand{\eat}[1]{}

\usepackage{geometry}
\geometry{a4paper,scale=0.8}
        {\hspace*{\fill}$\Box$\par\vspace{4mm}}
        {\hspace*{\fill}$\Box$\par}

\hypersetup{
    colorlinks=false,       %
    linkcolor=black,    %
    citecolor=black,        %
    filecolor=magenta,     %
    urlcolor=blue
}

\renewcommand{\paragraph}[1]{\noindent\textbf{#1}}

\title{Supplementary Materials of\\ Understanding the Impact of Adversarial Training on Accuracy Disparity}

\begin{document}

\maketitle

\input{sec_supp}

\end{document}
